# Supplementary material for: Effects of Parameter Norm Growth During Transformer Training: Inductive Bias from Gradient Descent
Source: arXiv:2010.09697 source file (2023-03-07)
Supplement: Supplementary file 1 [file new_dynamics_appendix.tex]

\section{Homogeneous Dynamics}

Let $\jac_\beta(g)$ be the Jacobian of a vector-valued function $g$ with respect to $\beta$. Let $y \in \{0, 1\}^v$ be a one-hot label vector. Note that $v$ can be thought of as the number of classes. Let $Z$ be the number of training examples $\langle x, y \rangle$. We write $f(\theta)$ for the mean of $f(x; \theta)$ over all $x$.

\begin{theorem}[Restates Proposition\ 1]
Assume standard GD for a $2$-homogeneous network $f$ with cross-entropy loss $L$. If
\begin{equation}
    \eta (1 - \alpha)^2 \min_i \norm{\nabla_{\theta_t} f_i}^2 > 16 \max_j \abs{ f_j(\theta_t) } ,
\end{equation}
then it holds that $\norm{\theta_t}$ is increasing at time $t$, i.e.
\begin{equation}
    \drho > 0 .
\end{equation}
\end{theorem}

\begin{proof}
For standard GD, we can write the GD expansion as
\begin{align}
    \drho
        &= \norm{\delta_t}^2 + 2 \theta_t^\top \cdot \delta_t \\
        &= \eta^2 \norm{\nabla_{\theta_t} L}^2 - 2 \eta \theta_t^\top \cdot \nabla_{\theta_t} L .
\end{align}
We first simplify the second term using the multivariate chain rule:
\begin{align}
    \theta_t^\top \cdot \nabla_{\theta_t} L
        &= \theta_t^\top \cdot \jac_{\theta_t}^\top(L) \\
        &= \theta_t^\top \cdot \jac_{\theta_t}^\top(f) \cdot \jac_f^\top(L) \\
        &= \theta_t^\top \cdot \jac_{\theta_t}^\top(f) \cdot \nabla_f L .
\end{align}
We leverage the homogeneity of $f$ and apply \autoref{thm:homo-grad}:
\begin{align}
    \theta^\top \cdot \nabla_{\theta_t} L
        &= f(\theta)^\top \cdot \nabla_f L \\
        &= f(\theta)^\top \cdot \left( \frac{1}{Z} \sum_{\langle x,y \rangle} \softmax(f(x; \theta)) - y \right) .
\end{align}
We can then bound the absolute value of the term as
\begin{align}
    &\abs{\theta^\top \cdot \nabla_{\theta_t} L} \\
        &= \abs{f(\theta)^\top \cdot \left( \frac{1}{Z} \sum_{\langle x,y \rangle} \softmax(f(x; \theta)) - y \right)} \\
        &\leq 2 \max_i \abs{f_i(\theta)} .
\end{align}
We now turn to the term $\norm{\nabla_{\theta_t} L}^2$.
\begin{align}
    \norm{\nabla_{\theta_t} L}^2
        &= \norm {\jac_f(L) \cdot \jac_{\theta_t}(f) }^2 \\
        &= \norm {\nabla_f^\top L \cdot \jac_{\theta_t}(f) }^2 \\
        &= \sum_{j=1}^n \sum_{i=1}^v \left( \pdv{L}{f_i} \pdv{f_j}{\theta_t^i} \right)^2 \\
        &= \sum_{i=1}^v \left( \pdv{L}{f_i} \right)^2 \sum_{j=1}^n \left( \pdv{f_j}{\theta_t^i} \right)^2 \\
        &= \sum_{i=1}^v \left( \pdv{L}{f_i} \right)^2 \cdot \norm{ \nabla_{\theta_t} f_i }^2 \\
        &\geq \norm{\nabla_f L}^2 \cdot \min_i \norm{ \nabla_{\theta_t} f_i }^2 \\
        &\geq \frac{1}{4} (1 - \alpha)^2 \cdot \min_i \norm{ \nabla_{\theta_t} f_i }^2 .
\end{align}
with the final line following from \autoref{thm:grad-lb}. We now put the two terms back together to get
\begin{align}
    \drho
        &\geq \eta^2 \cdot \frac{1}{4} (1 - \alpha)^2 \min_i \norm{ \nabla_{\theta_t} f_i }^2 \\
        &\quad \quad \quad - 2\eta \big(2 \max_j \abs{f_j(\theta)} \big) \\
        &\geq \eta^2 \cdot \frac{1}{4} (1 - \alpha)^2 \min_i \norm{ \nabla_{\theta_t} f_i }^2 - 4 \eta \max_j \abs{f_j(\theta)} .
\end{align}
We conclude that $\drho > 0$ when
\begin{equation}
    \eta (1 - \alpha)^2 \min_i \norm{ \nabla_{\theta_t} f_i }^2 > 16 \max_i \abs{f_i(\theta)} ,
\end{equation}
which is true by assumption in the theorem statement.
\end{proof}
